# Supplementary material for: Generating Adversarial Events: A Motion-Aware Point Cloud Framework
Source: arXiv:2602.08230 source file (2026-11-18)
Supplement: Supplementary file 1 [file X_suppl.tex]

\clearpage
\setcounter{page}{1}
\maketitlesupplementary


% \section{Rationale}
% \label{sec:rationale}
% % 
% Having the supplementary compiled together with the main paper means that:
% % 
% \begin{itemize}
% \item The supplementary can back-reference sections of the main paper, for example, we can refer to \cref{sec:intro};
% \item The main paper can forward reference sub-sections within the supplementary explicitly (e.g. referring to a particular experiment); 
% \item When submitted to arXiv, the supplementary will already included at the end of the paper.
% \end{itemize}
% % 
% To split the supplementary pages from the main paper, you can use \href{https://support.apple.com/en-ca/guide/preview/prvw11793/mac#:~:text=Delete%20a%20page%20from%20a,or%20choose%20Edit%20%3E%20Delete).}{Preview (on macOS)}, \href{https://www.adobe.com/acrobat/how-to/delete-pages-from-pdf.html#:~:text=Choose%20%E2%80%9CTools%E2%80%9D%20%3E%20%E2%80%9COrganize,or%20pages%20from%20the%20file.}{Adobe Acrobat} (on all OSs), as well as \href{https://superuser.com/questions/517986/is-it-possible-to-delete-some-pages-of-a-pdf-document}{command line tools}.
\section{Experimental Environment}
The main-paper experiments were performed on a machine with an AMD Ryzen 9 7950X CPU,
an NVIDIA RTX 4090 GPU, and 32\,GB of system memory, as stated in the main manuscript.
The digital white-box attacks were evaluated on PointNet, PointNet++, and EventMamba
using DVSGesture, N-Caltech101, and N-MNIST.
% VERIFY: The earlier supplementary draft instead states two Intel Xeon Gold 6430
% CPUs, one H100 PCIe 80GB GPU, 512GB RAM, CUDA 12.4 and driver 550.127.08.
% Check the actual experiment logs before attributing any measured runtimes to this hardware.


\section{ST-ADV Attack Generation}
\Cref{alg:stadv} summarizes the attack in the notation of the main manuscript.
Let $\mathcal E=\{e_i\}_{i=1}^N$ with $e_i=(x_i,y_i,t_i,p_i)$ and
$\mathbf X\in\mathbb R^{N\times 3}$ denote the spatio-temporal coordinates.
The trainable perturbation $\mathbf P\in\mathbb R^{N\times3}$ changes only
$(x,y,t)$; all event polarities are preserved. The spatial and temporally
ordered KNN neighborhoods are computed from the input event stream.
Both KNN searches use distances in the joint $(x,y,t)$ space, while
$\mathrm{KNN}_t$ considers only events occurring after the current event.

For consecutive events, let $\Delta\mathbf s_i=(x_i-x_{i-1},y_i-y_{i-1})$ and
$\Delta t_i=t_i-t_{i-1}$. The variation cue used in the temporal branch is
\begin{equation}
\mathbf v_i=\begin{cases}
\operatorname{clip}(\Delta\mathbf s_i/\Delta t_i,-v_{\max},v_{\max}),&|\Delta t_i|\ge\tau,\\
\mathbf0,&\text{otherwise},
\end{cases}\label{eq:sup_variation}
\end{equation}
where $\tau=\max(10^{-6},0.01m_t)$, $m_t$ is the median nonzero
absolute timestamp difference in the current mini-batch
($m_t=10^{-3}$ when none exists), and
$v_{\max}=\min(2Q_{0.95}/\tau,1000)$.
Here $Q_{0.95}$ is the 95th percentile of consecutive spatial
 displacement magnitudes in the mini-batch.
For the first event, $\mathbf v_1=\mathbf 0$. The normalized cue is
\begin{equation}
\mathcal C_i=\begin{cases}
\|\mathbf v_i\|_2/V_{\max},&V_{\max}>0,\\
0,&\text{otherwise},
\end{cases}\quad V_{\max}=\max_i\|\mathbf v_i\|_2,
\label{eq:sup_cue}
\end{equation}
with the maximum evaluated over the current mini-batch; $\mathcal C_1=0$.
The event-wise cues are assembled into a temporal variation matrix
$\mathbf V$ as described in the main text.
% VERIFY: Specify the exact construction of V_{ij} from C_i using the actual code.
% In particular, broadcast rows V_{ij}=C_i would give approximately uniform
% normalized temporal-neighbor weights; matrix notation does not resolve that.

The diffusion weights match Eq.~(13) of the main paper:
\begin{equation}
\mathbf W_s=\exp\!\left(-\frac{\mathbf D^{\odot2}}{\sigma_s}\right),\qquad
\mathbf W_t=\exp\!\left(-\frac{\mathbf V}{\sigma_t}\right),
\label{eq:sup_weights}
\end{equation}
where $\mathbf D$ collects the corresponding joint spatio-temporal KNN
distances, $\odot2$ denotes element-wise squaring, and the exponential is
applied element-wise. Each weight set is normalized within its own
neighborhood using a small $\varepsilon>0$ in the denominator.
We denote the resulting normalized weights by $\bar w^r_{ij}$,
$r\in\{s,t\}$. The residual diffusion step is
\begin{equation}
\widetilde{\mathbf p}_i
=\mathbf p_i+\frac12\sum_{r\in\{s,t\}}
\sum_{j\in\mathcal I_r(i)}\bar w^r_{ij}\mathbf p_j.
\label{eq:sup_diffusion}
\end{equation}
This includes the original perturbation $\mathbf p_i$, unlike a pure
average of neighboring perturbations.

\begin{algorithm*}[t]
\caption{ST-ADV: spatio-temporal adversarial event generation}
\label{alg:stadv}
\begin{algorithmic}[1]
\REQUIRE Correctly classified input $\mathcal E$, label $y$, victim $f_\theta$;
$J$ binary-search steps, $I$ iterations, neighborhood size $K$
\ENSURE Adversarial event stream $\mathcal E'$ (if a successful perturbation exists)
\STATE Extract $\mathbf X$ and unchanged polarities $\mathbf p^{\rm pol}$ from $\mathcal E$
\STATE $(\mathcal I_s,\mathbf D)\leftarrow\mathrm{KNN}_s(\mathcal E,K)$;
$\mathcal I_t\leftarrow\mathrm{KNN}_t(\mathcal E,K)$
\STATE Compute $\{\mathbf v_i,\mathcal C_i\}$ using \cref{eq:sup_variation,eq:sup_cue}
\STATE Construct $\mathbf V$; compute and normalize $\mathbf W_s,\mathbf W_t$
\STATE Initialize sample-wise binary-search bounds $\lambda_l=0$, $\lambda_h=80$
\STATE Initialize record of lowest-distortion successful candidate $\mathbf P^*$
\FOR{$j=1$ to $J$}
    \STATE Select $\lambda^{(j)}$ from the current binary-search bounds
    \STATE $P^{(0)}_{n,d}\sim \mathcal U(0,10^{-7})$ independently
    \STATE Initialize Adam moments and sample-wise $\eta^{(0)}[k]=\eta_0$
    \FOR{$q=0$ to $I-1$}
        \STATE $\mathbf X_{\rm adv}^{(q)}\leftarrow\mathbf X+\mathbf P^{(q)}$
        \STATE Evaluate $\mathcal L_{\rm total}=\mathcal L_{\rm adv}+\lambda^{(j)}\mathcal L_{\rm distance}$
        \STATE $\mathbf G^{(q)}\leftarrow\nabla_{\mathbf P^{(q)}}\mathcal L_{\rm total}$
        \STATE Update sample-wise $\eta^{(q)}[k]$ from attack status (every $h$ steps)
        \STATE $\widehat{\mathbf P}^{(q+1)}\leftarrow\operatorname{AdamStep}(\mathbf P^{(q)},\mathbf G^{(q)},\eta^{(q)})$
        \STATE Apply residual neighborhood diffusion \cref{eq:sup_diffusion} to $\widehat{\mathbf P}^{(q+1)}$
        \STATE Set $\mathbf P^{(q+1)}$ to the diffused perturbation, respecting valid input ranges
        \STATE Record successful candidates with smaller distortion
    \ENDFOR
    \STATE Update each sample's $\lambda_l,\lambda_h$ according to attack success
\ENDFOR
\STATE Reconstruct $\mathcal E'$ from $\mathbf X+\mathbf P^*$ and $\mathbf p^{\rm pol}$
\RETURN $\mathcal E'$
\end{algorithmic}
\end{algorithm*}
% VERIFY: The update/diffusion ordering above follows the source SI sequence
% while adding the residual in the CVPR Eq.(14); confirm it matches the actual code.
% VERIFY: Clarify behavior when no successful candidate is found and how clipping/projection
% is handled (in optimization and/or postprocessing).

The untargeted logit-margin loss, directed distance regularizer,
and sample-wise learning-rate adaptation use the definitions
reported in the main manuscript (Eqs.~(17)--(22)). We restate the
optimization objective as
\begin{equation}
\mathcal L_{\rm total}(\mathcal E',y)
=\mathcal L_{\rm adv}(\mathcal E',y)
+\lambda\mathcal L_{\rm distance}(\mathbf X',\mathbf X),
\label{eq:sup_objective}
\end{equation}
where
\begin{align}
\mathcal L_{\rm adv}
&=\frac1B\sum_{b=1}^{B}\max\!\left(z_b(y_b)-\max_{c\ne y_b}z_b(c)+\kappa,0\right),\\
\mathcal L_{\rm distance}
&=\frac1N\sum_{i=1}^{N}\min_{j\in\{1,\ldots,N\}}
\|\mathbf x'_i-\mathbf x_j\|_2.
\label{eq:sup_distance_loss}
\end{align}
The loss is minimized for untargeted misclassification. The binary-search
weight $\lambda$ is sample-specific; $B$ is the batch size and $\kappa\ge0$
the confidence margin.


\section{Runtime Analysis}
Under the same setting with 20 binary-search steps and 100 optimization iterations, ST-ADV requires 28.8002s per attack, which is comparable to C\&W (28.9944s), HIT-ADV (28.3701s), and $\text{GeoA}^3$ (28.6511s). Although ST-ADV introduces additional spatio-temporal perturbation diffusion and sample-wise adaptive optimization, these components only involve lightweight neighborhood aggregation and learning-rate adjustment operations, resulting in negligible extra computational overhead. The overall runtime is still dominated by the iterative forward-backward optimization process and binary search procedure used to balance attack effectiveness and perturbation cost. Compared with existing optimization-based attacks, ST-ADV achieves improved perturbation efficiency and event-level spatio-temporal consistency without increasing the computational burden.

This result further demonstrates that the proposed motion-aware design provides an effective trade-off between attack quality and computational efficiency. In particular, the diffusion operation only performs local information propagation among pre-computed event neighbors, avoiding expensive global optimization or additional network inference. Meanwhile, the sample-wise learning rate adjustment is integrated into the existing Adam update process without introducing extra gradient computation. Therefore, ST-ADV can maintain similar execution efficiency while generating adversarial events with lower distortion and stronger robustness against defensive preprocessing, making it suitable for practical robustness evaluation of event-based perception systems.


% The original supplementary source references curve.jpg but did not provide the asset.
% VERIFY: The curve must be regenerated or checked against ST-ADV labels/results.
\IfFileExists{curve.jpg}{%
\begin{figure*}[t]
\centering
\includegraphics[width=\textwidth]{curve.jpg}
\caption{Attack success rate versus perturbation distortion for the
compared attacks. The figure illustrates geometric and event-specific
distortion trade-offs under the indicated attack budgets.}
\label{fig:stadv_tradeoff}
\end{figure*}
}{}


\section{Evaluation Metrics}
We evaluate the success of untargeted digital white-box attacks
and the distortion of the resulting adversarial event streams.
Throughout this section, $\mathbf x_i=(x_i,y_i,t_i)$ and
$\mathbf x'_i=(x'_i,y'_i,t'_i)$ denote continuous spatio-temporal
coordinates; polarity $p_i$ is unchanged and is not included in
these distance calculations.

\paragraph{Success Rate (SR).}
Let $\mathcal S$ denote the set of evaluation samples that the victim
classifies correctly before attack. Then
\begin{equation}
\mathrm{SR}=
\frac{1}{|\mathcal S|}\sum_{b\in\mathcal S}
\mathbb I\!\left[\arg\max_c f_\theta(\mathcal E'_b)_c\ne y_b\right].
\label{eq:sup_sr}
\end{equation}
A larger SR indicates a more effective untargeted attack.

\paragraph{Geometric distortion.}
This geometric metric uses the following directed
nearest-neighbor distance from adversarial to original events as its
Chamfer-type evaluation metric:
\begin{equation}
D_{\rm Chamfer}(\mathbf X,\mathbf X')=
\frac1N\sum_{i=1}^{N}\min_{j}
\|\mathbf x'_i-\mathbf x_j\|_2.
\label{eq:sup_chamfer}
\end{equation}

The average event-wise $L_2$ displacement is
\begin{equation}
D_{L_2}(\mathbf X,\mathbf X')=
\frac1N\sum_{i=1}^{N}\|\mathbf x'_i-\mathbf x_i\|_2,
\label{eq:sup_l2}
\end{equation}
and the symmetric Hausdorff distance is
\begin{equation}
\begin{split}
D_{\rm Hausdorff}(\mathbf X,\mathbf X')=\max\{&
\max_i\min_j\|\mathbf x_i-\mathbf x'_j\|_2,\\
&\max_j\min_i\|\mathbf x'_j-\mathbf x_i\|_2\}.
\end{split}
\label{eq:sup_hausdorff}
\end{equation}
% VERIFY: Check whether the implemented D_L2 is average event-wise
% displacement, global Frobenius/L2 norm, or another reduction.

\paragraph{Normalized Temporal Perturbation (NTP).}
As in Eq.~(23) of the main manuscript,
\begin{equation}
\mathrm{NTP}(\mathcal E,\mathcal E')=
\frac1N\sum_{i=1}^N
\frac{|t'_i-t_i|}{t_{\max}-t_{\min}+\varepsilon}.
\label{eq:sup_ntp}
\end{equation}
Here $t_{\max}$ and $t_{\min}$ are determined from the original event
window. Lower NTP indicates smaller average timestamp perturbations.

\paragraph{Temporal Surface Consistency (TSC).}
The original supplemental metric uses a polarity-agnostic
exponentially decayed time surface. For pixel $(u,v)$ and a
specified polarity, let $t_{u,v}$ be the timestamp of the most recent
event and $t_{\rm ref}$ the reference timestamp for the window.
The surface is defined as
\begin{equation}
S_{\mathcal E}(u,v)=\exp\!\left(
-\frac{t_{\rm ref}-t_{u,v}}{\tau_{\rm surf}}\right),
\label{eq:sup_surface}
\end{equation}
where $\tau_{\rm surf}>0$ is the time-surface decay parameter
(distinct from the threshold $\tau$ in \cref{eq:sup_variation}).
Surfaces for the two polarities are computed separately and averaged.
At the original sensor resolution, $\Omega^+$ denotes the set of pixels
containing at least one event in either stream. The TSC is
\begin{equation}
\mathrm{TSC}(\mathcal E,\mathcal E')=
\frac1{|\Omega^+|}\sum_{(u,v)\in\Omega^+}
\left|S_{\mathcal E}(u,v)-S_{\mathcal E'}(u,v)\right|.
\label{eq:sup_tsc}
\end{equation}
Smaller TSC reflects closer time-surface representations.
% VERIFY: Specify how pixels with no event for one polarity are handled,
% reference timestamp and decay parameter values, and whether spatial
% event positions are discretized/rounded before the surface computation.


\section{Attack Efficiency Analysis}
The main paper reports that ST-ADV obtains $100\%$ success rates across
three event datasets and three victim models, while improving the
Chamfer and $L_2$ distortion measures over the C\&W baseline in those
nine settings. Event-aware comparisons based on NTP and TSC provide
additional evidence that the resulting attacks typically preserve
more temporal structure under the chosen metrics.

% If curve.jpg is present, the following reference is enabled in the build.
\IfFileExists{curve.jpg}{The success-rate/distortion trade-off curves
are provided in \cref{fig:stadv_tradeoff}.}{}
The reported comparisons support the empirical effectiveness of
spatio-temporal perturbation aggregation. They do not, by themselves,
prove that individual gradient fluctuations are suppressed or that
physical motion trajectories are preserved; those would require
additional direct measurements.


\subsection{Sample-wise Adaptive Optimization}
The sample-wise learning-rate mechanism is intended to improve
optimization reliability across events of different difficulty,
rather than acting as the primary distortion regularizer.
Let $s^{(q)}[k]\in\{0,1\}$ indicate attack success for sample $k$
at iteration $q$. With initial rate $\eta^{(0)}[k]=\eta_0$, the
learning rate is updated at every $h$-th iteration:
\begin{align}
\rho^{(q)}[k]&=a\,s^{(q)}[k]+b(1-s^{(q)}[k]),\\
\eta^{(q)}[k]&=\begin{cases}
\eta^{(q-1)}[k]\rho^{(q)}[k],&q\bmod h=0,\\
\eta^{(q-1)}[k],&\text{otherwise},
\end{cases}
\label{eq:sup_adaptive}
\end{align}
where $a=0.8<1$ and $b=1.2>1$ in the main-paper experiments.
Successful samples receive smaller learning-rate updates; unsuccessful
samples receive larger ones. This procedure modifies the Adam step
size, not its first- and second-moment definitions.

The ablation in the main paper shows that removing adaptive learning
rate modestly increases Chamfer and $L_2$ distortions, while the effect
on Hausdorff distance is mixed. Hence, its main documented role is an
optimization refinement rather than an independent guarantee of
smaller distortion on every metric.
% VERIFY: The earlier supplementary draft asserted that unsuccessful attacks receive zero
% distortion in averages. This must be verified against the evaluation
% code and clearly disclosed if true; zero-fill can bias means downward.


\section{Graph Interpretation of Perturbation Diffusion}
\subsection{Event Neighborhood Graphs}
A graph view provides an interpretation of the neighborhood
aggregation used by ST-ADV. Let $\mathcal G_s=(\mathcal V,\mathcal E_s)$
and $\mathcal G_t=(\mathcal V,\mathcal E_t)$ denote graphs induced by
the spatial and temporally ordered KNN neighborhoods, respectively.
The two graphs both use the joint spatio-temporal distance for
neighbor retrieval; the temporal graph additionally imposes an
ordering constraint on its candidate neighbors.

The corresponding edge weights are obtained from
\cref{eq:sup_weights}, namely
\begin{equation}
w_{ij}^{s}=\exp(-d_{ij}^2/\sigma_s),\qquad
w_{ij}^{t}=\exp(-V_{ij}/\sigma_t),
\label{eq:sup_graph_weights}
\end{equation}
where $d_{ij}$ is the joint $(x,y,t)$ neighbor distance and $V_{ij}$
is the entry of the event-variation matrix in the temporal branch.
These formulas are not based on an independently estimated optical flow
or pairwise apparent-motion discrepancy. Their normalized versions
$\bar w^r_{ij}$ are those used for diffusion.

A standard graph smoothness penalty can be used as a conceptual
reference. Since the temporal neighborhood may be directed, define
a \emph{symmetric surrogate} adjacency
$A^r_{ij}=(\bar w^r_{ij}+\bar w^r_{ji})/2$,
where absent edges have zero weight. Then
\begin{equation}
\mathcal R(\mathbf P)=\frac14\sum_{r\in\{s,t\}}
\sum_{i,j} A^r_{ij}\|\mathbf p_i-\mathbf p_j\|_2^2.
\label{eq:sup_smoothness}
\end{equation}
For this symmetric surrogate, the gradient is
\begin{equation}
\nabla_{\mathbf p_i}\mathcal R(\mathbf P)
=\sum_{r\in\{s,t\}}\sum_j
A^r_{ij}(\mathbf p_i-\mathbf p_j).
\label{eq:sup_graph_gradient}
\end{equation}
This expression illustrates how a graph regularizer would encourage
neighboring perturbations to become similar. It is provided only as
an interpretation: ST-ADV does \emph{not} explicitly add
$\lambda_r\mathcal R$ to the attack objective in the main paper.

\subsection{Residual Neighborhood Propagation}
The actual ST-ADV diffusion in the main paper is the residual
aggregation of \cref{eq:sup_diffusion}:
\begin{equation}
\widetilde{\mathbf P}=
\left(\mathbf I+\frac12(\bar{\mathbf W}_s+
\bar{\mathbf W}_t)\right)\mathbf P,
\label{eq:sup_graph_filter}
\end{equation}
where the two sparse normalized matrices are padded with zeros
outside their respective neighborhoods. This operation constitutes
a local message-passing step and couples perturbations across related
events, but it is not algebraically identical to a gradient-descent
step on \cref{eq:sup_smoothness}. In particular, its residual form
is not guaranteed to reduce an arbitrary graph high-frequency energy
without additional assumptions. Consequently, the graph view is
an intuitive motivation, not a formal equivalence proof.

\subsection{Relationship to Adaptive Optimization}
ST-ADV combines event-neighborhood coupling with the sample-wise
Adam learning-rate adjustment in \cref{eq:sup_adaptive}. The two
components play different roles: local aggregation changes the
structure of the coordinate perturbation field, while sample-wise
step sizes adjust the optimization trajectory based on attack success.
Together, they provide a practical framework for balancing attack
success and distortion within the digital white-box threat model.


\begin{table*}[t]
\centering
\caption{High-level comparison of the attack strategies considered in this work.
The descriptions of prior attacks summarize their design principles rather than
reproducing every implementation detail.}
\label{tab:attack_comparison}
\begin{tabular}{lll}
\toprule
Method & General strategy & Main update/constraint \\
\midrule
FGSM & Single-step gradient attack & Signed cross-entropy gradient \\
IFGSM & Iterative gradient attack & Repeated signed-gradient updates \\
C\&W & Optimization-based attack & Margin loss and distortion regularization \\
HIT-ADV & Geometry-aware point-cloud attack & Structure-aware imperceptibility constraints \\
ST-ADV & Spatio-temporal event attack & Residual neighborhood diffusion and adaptive Adam \\
\bottomrule
\end{tabular}
\end{table*}


\section{Adversarial Attack Baselines}
\Cref{tab:attack_comparison} summarizes the broad optimization
strategies of FGSM, IFGSM, C\&W, HIT-ADV, and ST-ADV.
These methods address different perturbation and optimization regimes;
comparisons should use matched targets and explicitly reported budgets.

\subsection{Fast Gradient Sign Method (FGSM)~\cite{goodfellow2014explaining}}
FGSM takes a single untargeted step that increases a classification
loss, such as cross-entropy $\ell_{\rm CE}$:
\begin{equation}
\mathbf X'=\mathbf X+
\epsilon_{\rm attack}\operatorname{sign}
\left(\nabla_{\mathbf X}\ell_{\rm CE}(f_\theta(\mathcal E),y)\right).
\label{eq:sup_fgsm}
\end{equation}
Only the continuous event coordinates are modified in this digital
point-based setting, and polarities are left unchanged. The step size
$\epsilon_{\rm attack}$ controls the magnitude of the update.

\subsection{Iterative FGSM (IFGSM)~\cite{liu2019extending}}
IFGSM applies repeated untargeted sign-gradient updates:
\begin{equation}
\mathbf X^{(q+1)}=\mathbf X^{(q)}+
\alpha\operatorname{sign}\left(
\nabla_{\mathbf X^{(q)}}\ell_{\rm CE}(f_\theta(\mathcal E^{(q)}),y)
\right).
\label{eq:sup_ifgsm}
\end{equation}
The precise step count and any projection/clipping operator are part
of the baseline implementation and should be reported for a fair
comparison; \cref{eq:sup_ifgsm} is a schematic update.

\subsection{Carlini--Wagner (C\&W)~\cite{xiang2019generating}}
A C\&W-style formulation minimizes a logit-based untargeted margin
loss together with a distortion penalty:
\begin{equation}
\min_{\mathbf P}\ \mathcal L_{\rm adv}(\mathbf X+\mathbf P,y)
+\lambda\mathcal D(\mathbf X+\mathbf P,\mathbf X),
\label{eq:sup_cw}
\end{equation}
where $\mathcal D$ is the chosen point-set distance and
$\mathcal L_{\rm adv}$ is the margin loss in \cref{eq:sup_objective}.
This is a high-level formulation rather than a claim that every C\&W
baseline uses exactly the ST-ADV loss or regularizer.

\subsection{HIT-ADV~\cite{lou2024hide}}
HIT-ADV uses geometry-aware constraints to generate low-distortion
adversarial point clouds. Its constraints prioritize static geometric
structure, whereas ST-ADV also leverages the temporal organization
of the asynchronous events. For reproducibility, the baseline
configuration should be taken from the implemented version of
HIT-ADV, rather than approximated by an unverified equation.

\subsection{ST-ADV}
Our attack optimizes the coordinates $\mathbf X$ of individual events
while leaving their polarities unchanged. It constructs two
spatio-temporal neighborhood systems, forms exponential diffusion
weights from joint coordinate distances and normalized local variation
cues, and performs residual perturbation aggregation as in
\cref{eq:sup_diffusion}. The sample-wise Adam learning rate is updated
based on attack status as in \cref{eq:sup_adaptive}.
\Cref{alg:stadv} provides the full operational summary.

\paragraph{Existing event-based attacks.}
Earlier event adversarial approaches, such as
\citet{lee2022adversarial} and \citet{buchel2022adversarial},
operate under different event manipulation spaces, such as timestamp
changes, event insertion or removal, or spiking-network settings.
Their reported success rates may be informative as context but are not
directly comparable to the point-based white-box evaluation in this
work without matching the victim models, sample sets, and perturbation
budget. The event-aware NTP and TSC metrics further require a specified
representation and correspondence between original and adversarial
event streams.


% VERIFY: Reuse the same .bib database as the main CVPR manuscript.
% This file references main.bib; change the filename if your project uses a different name.
{\small
\bibliographystyle{ieeenat_fullname}
\bibliography{main}
}
